# Supplementary material for: TAPE: Tailored Posterior Difference for Auditing of Machine Unlearning
Source: arXiv:2502.19770 source file (2025-03-17)
Supplement: Supplementary file 4 [file appendix4.tex]

\subsection{Batched Time Analysis of Sharding}
\label{appendix:time_sharding_batch}

\noindent{\em Proof:} Let $S$ denote the number of shards and $K$ the number of points in the batch.
Let $(\mathfrak{s}_i)_{i \in \{1,\dots,K\}}$ be random variables that give the index of the shard impacted by each point in the batch. We assume that those variables are i.i.d. and that:
\[\forall i \in \{1,\dots,K\}, \mathfrak{s}_i \sim U(0, S)\]
We can define $(\mathfrak{h}_j)_{j \in \{1,\dots,S\}}$ which are Bernoulli random variables whose value is 1 when shard $j$ is impacted.
We have:

{\small\[\mathfrak{h}_j = 0 \Longleftrightarrow \forall i \in \{1,\dots,K\}, \mathfrak{s}_i \ne j\]}

Thus $\mathbb{P}(\mathfrak{h}_j = 0) = \left(1 - \frac{1}{S}\right)^K$. We define the total cost $C$ of retraining as the number of points that need to be retrained while processing the batch as $C = \sum_{j=1}^S\mathfrak{h}_j|\mathcal{D}_j|$

To obtain $|\mathcal{D}_j|$, we define $(\mathfrak{u}_j)_{j \in \{1,\dots,K\}}$, the random variables that count the number of times each shard is affected. These variables count the number of successes in a repetition of independent Bernoulli experiments, namely counting the number of times $\mathfrak{s}_i = j$, when $i$ varies from $1$ to $K$. Thus:
{\small\[\forall j \in \{1,\dots,S\}, \mathfrak{u}_j \sim B\left(K, \dfrac{1}{S}\right)\]}

{\small\begin{equation}\begin{aligned}
C &= \sum_{j=1}^S{\mathfrak{h}_j\left(\frac{N}{S} - \mathfrak{u}_j\right)}
&= \sum_{j=1}^S{\left(\frac{N\mathfrak{h}_j}{S} - \mathfrak{u}_j\mathfrak{h}_j\right)}
\end{aligned}\end{equation}}
By construction,
{\small\[\mathfrak{h}_j = 0 \Longleftrightarrow \mathfrak{u}_j = 0\]}
Thus $\mathfrak{u}_j\mathfrak{h}_j = \mathfrak{u}_j$ and:
{\small\[C = \sum_{j=1}^S{\left(\frac{N\mathfrak{h}_j}{S} - \mathfrak{u}_j\right)}\]}
Using the linearity of the expected value and the expected values of Bernouilli and binomial random variables,
{\small\begin{equation}\begin{aligned}
\mathbb{E}[C] &=& \sum_{j=1}^S{\left(\frac{N}{S}\left(1-\left(1-\frac{1}{S}\right)^K\right) - \frac{K}{S}\right)}\\
&=& N\left(1-\left(1-\frac{1}{S}\right)^K\right) -K
\end{aligned}\end{equation}}
