# Supplementary material for: TAPE: Tailored Posterior Difference for Auditing of Machine Unlearning
Source: arXiv:2502.19770 source file (2025-03-17)
Supplement: Supplementary file 5 [file appendix5.tex]

\subsection{Sequential Time Analysis of Slicing}
\label{appendix:time_slicing_sequential}

\noindent{\em Proof:} When a model is trained on an entire shard (\ie without slicing) of size $D=\frac{N}{S}$ for $e'$ epochs, the number of samples seen by the training algorithm is proportional to $e'D$.
Recall from \S~\ref{sec:approach} that we modified the number of epochs $e$ when slicing is applied (refer to equation~\ref{eq:slice_epoch}).
For each slice indexed $r$, we use data from the first $r$ slices (\ie $\frac{rD}{R}$ samples), training the model for $\frac{2e'}{R+1}$ epochs. Therefore, if an unlearning request hits the $r^{th}$ slice, we need to retrain the model from the $r^{th}$ slice to the $R^{th}$ slice, leading to the following retraining cost (\ie number of samples):

{\small\begin{equation}\begin{aligned}
    C &= \sum_{j = r}^R{\frac{2e'}{R+1}\frac{jD}{R}}
    &= \frac{2e'D}{R(R+1)}\left(\frac{R(R+1)}{2} - \frac{r(r-1)}{2}\right)
\end{aligned}\end{equation}}

We model the index of a slice hit by an unlearning request by the random variable $\mathfrak{r} \sim U(\{1,\dots,R\})$.
The expected cost can be expressed as:
{\small\begin{equation}\begin{aligned}
    \mathbb{E}[C] 
    &= \frac{2e'D}{R(R+1)}\left(\frac{R(R+1)}{2} - \frac{1}{2}\left(\mathbb{E}[\mathfrak{r}^2] - \mathbb{E}[\mathfrak{r}]\right))\right)
\end{aligned}\end{equation}}
We can compute the two first moments of $\mathfrak{r}$:

{\small\[\begin{array}{lclcl}
    \mathbb{E}[\mathfrak{r}] &=& \sum_{k=1}^R{k\mathbb{P}(\mathfrak{r}=k)} &=& \frac{R+1}{2}\\
    \mathbb{E}[\mathfrak{r}^2] &=& \sum_{k=1}^R{k^2\mathbb{P}(\mathfrak{r}=k)} &=& \frac{(R+1)(2R+1)}{6}\\
\end{array}\]}

And plug them into the expected cost:
{\small\begin{equation}\begin{aligned}
    \mathbb{E}[C] &= \frac{e'D}{R}\left(R - \frac{2R + 1}{6} + \frac{1}{2}\right)
    &= e'D\left(\frac{2}{3} + \frac{1}{3R}\right)\\
\end{aligned}\end{equation}}
\new{Note that for $R > 20$, the speed-up starts to plateau and any increase in $R$ does not provide a significant speed-up gain.}
