# Supplementary material for: TAPE: Tailored Posterior Difference for Auditing of Machine Unlearning
Source: arXiv:2502.19770 source file (2025-03-17)
Supplement: Supplementary file 9 [file appendix9.tex]

\subsection{Impact of number of samples per class on learnability}
\label{appendix:samples_per_class}
\new{The results from Figure~\ref{fig:miniimagenet_frac_dataset_accuracy} suggest that as the number of samples per class goes down, so does the accuracy.  This is the case with increased sharding for complex learning tasks.}

\begin{figure}[h]
\centering
{\includegraphics[width=.6\linewidth]{Figures/miniimagenet_data_acc.pdf}}  
\caption{\small \new{We plot the test accuracy as a function of the average number of samples per class. Observe that as the average number of samples per class increases, so does the accuracy.}} 
\label{fig:miniimagenet_frac_dataset_accuracy}
\end{figure}
